# Supplementary material for: Formation of motile cell clusters in heterogeneous model tumors: the role of cell-cell alignment
Source: arXiv:2406.14196 source file (2024-10-17)
Supplement: Supplementary file 1 [file S1_File_SupplementaryInformation.pdf]

# Supplementary Information (SI)

The information provides additional support for the main claims in the paper "Formation of motile cell clusters in heterogeneous model tumors: the role of cell-cell alignment" by Quirine J.S. Braat, Cornelis Storm and Liesbeth M.C. Janssen.

## Parameter estimation

To get an estimate for the typical values of the cells and their dynamics in the simulations, we use information about the dynamics of breast cancer cells in dense tissue [1,2]. A typical area of such breast cancer cells is 400 µm$^2$ and therefore the size of a pixel in the simulation is 2 µm by 2 µm. To determine the typical timescale, we can use the characteristic velocity of cells. In the CPM, velocities are an emerging quantity thus the velocities of the migrating cells are not constant but distributed around a mean, as is the case for cells in a dense confluent layer [2,3]. Typical velocities of breast cancer cells can vary considerably (ranging from 0.2 µm/min for non-invasive MCF7 to 0.7 µm/min for invasive MDA-MB-231 [2]). In the simulations, the mean velocity of the active mesenchymal cells ($\approx 0.03$ pixels/mcs) is significantly larger than the epithelial cells ($\approx 0.015$ pixels/mcs), see Fig. S1. Comparing our active cell velocities with the typical experimental velocities of more invasive phenotypes, e.g. 5.0 µm/min), we estimate the time scale of 1 mcs to represent approximately 7 seconds.

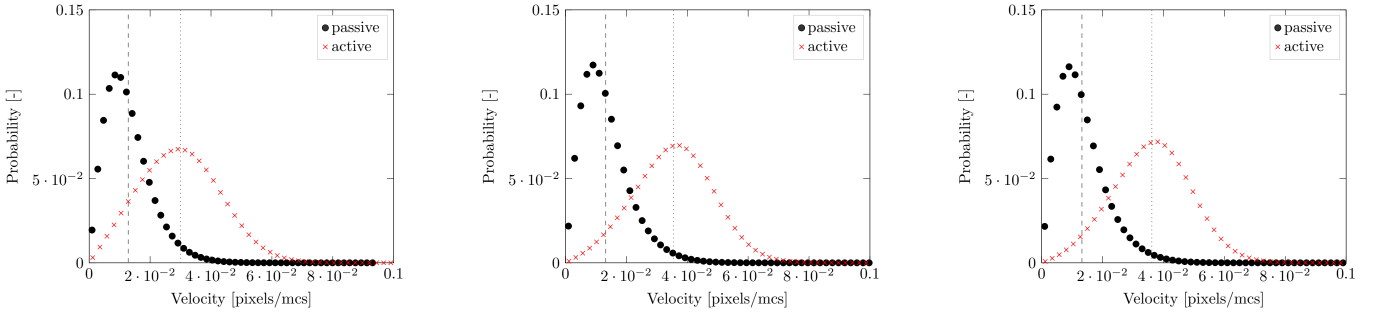


(a) (b) (c)

Figure S1: The velocity distribution of the active (motile) and passive (non-motile) cells for $\gamma = 0.01$ and $\tau = 500$ mcs (a), $\tau = 2500$ mcs (b) and $\tau = 4000$ mcs (c). The mean velocities are indicated by the gray lines. The active cells have a larger mean velocity and the distribution is wider. The curves are similar to the distributions observed in [2] where more mesenchymal-like cells migrate faster compared to more epithelial-like cells.

## Steady state

The analysis in the main text focuses on the dynamics starting from a random configuration where both the cells and the active force directions are randomly distributed with a uniform distribution. To verify whether the steady state is dependent on the initial configuration, we initiated the simulations with the same number of 400 motile cells, but now placed as a rectangular cluster of 20 by 20 cells in the center of the box. Once the active force is turned on, all cells initially move in the same direction, thus forming a strongly aligned cluster at the start. We run these simulations with the same update rules as in the protocol described in the main text, allowing cells to decorrelate in time. The time evolution of the mean cluster size converges towards a steady state value, see Fig. S2, and the final steady state value is identical for the different initial conditions. The latter result is shown in Fig. S3. The steady state value is thus a property of the alignment strength and cellular environment, and does not depend on the two extreme initial conditions.

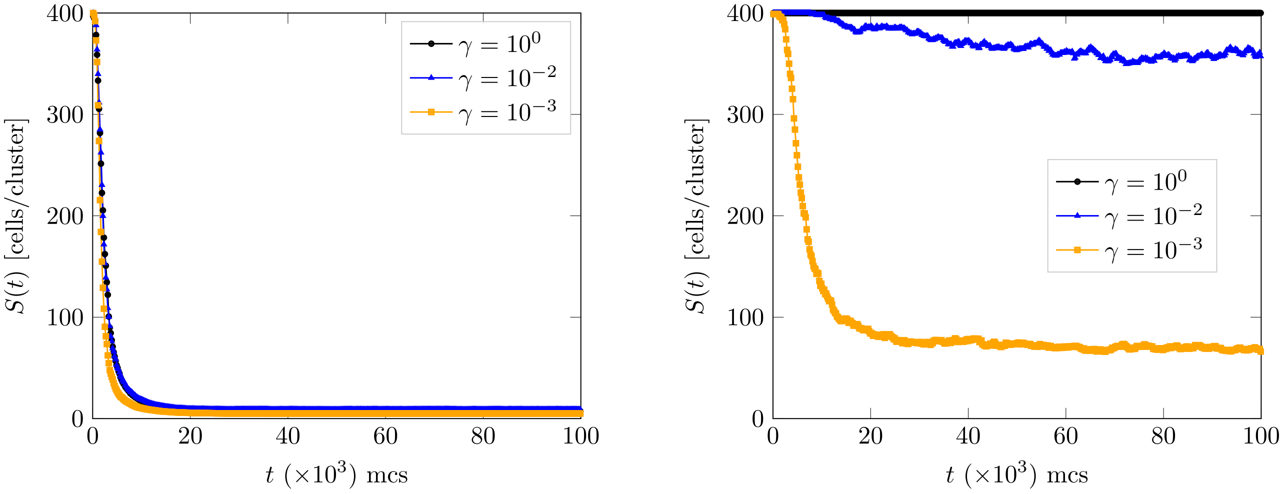


(a) (b)

Figure S2: The time evolution of the mean cluster size for $\gamma = 1.0$ (black, circles), $\gamma = 10^{-2}$ (blue, triangle) and $\gamma = 10^{-3}$ (yellow, square) in the confluent layer (a) and the empty layer (b). The layer is initiated with one fully aligned cluster with 400 motile cells. The simulations are run for $\tau = 2500$. and reaches a steady state.

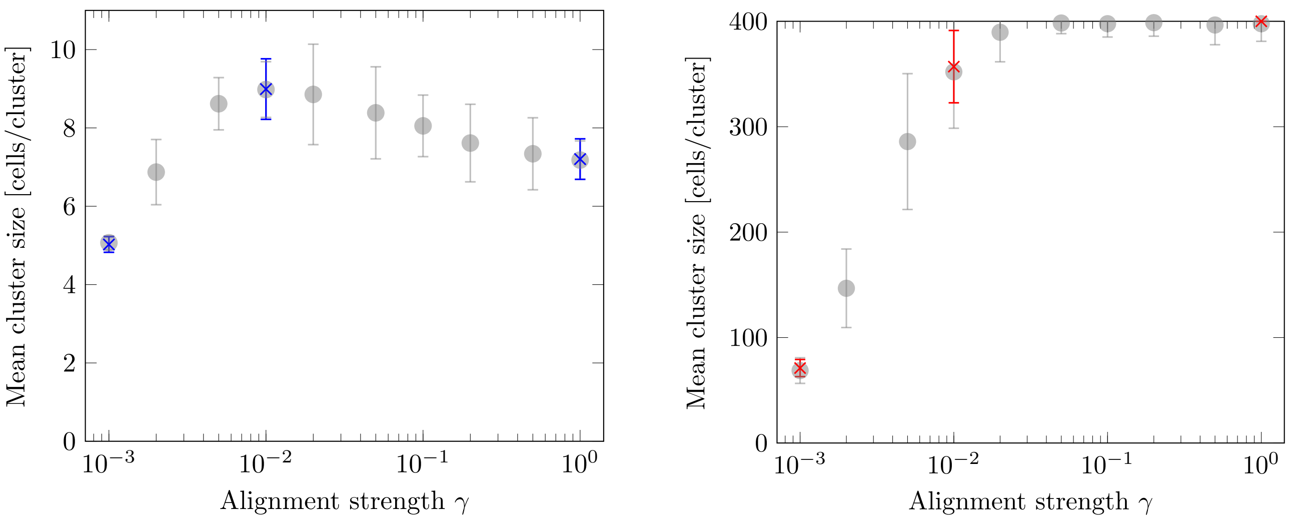


(a) (b)

Figure S3: Steady state mean cluster size for (a) the confluent cell layer and (b) the free space condition. The mean cluster size is plotted as a function of the alignment strength for the random initial condition (in gray, introduced in the main text) and the initial strongly aligned cluster (colored symbols for three different $\gamma$). The results are compared for a persistence time $\tau = 2500$ mcs. The steady state mean cluster size does not depend on the initial condition.

## Finite-size effects

To check for the effect of the box size, we ran simulations for $100, 400, 900, 1600, 2500$ cells in the simulation and calculated the mean cluster size for all different systems. Fig. S4 shows the time evolution for the mean cluster size for the various system sizes. As the number of cells in the simulation increases, the mean cluster size seems to approach a constant value. To get an estimate for the expected steady state mean cluster size in the limit of $N \to \infty$ (number of

cells approaching infinity), we fitted the function $S_\infty(N) = C - A\exp(-N/B)$ where $C$ is the expected steady state. We find this value to be $9.3 \pm 0.9$, which is relatively close to the value we find for 1600 cells.

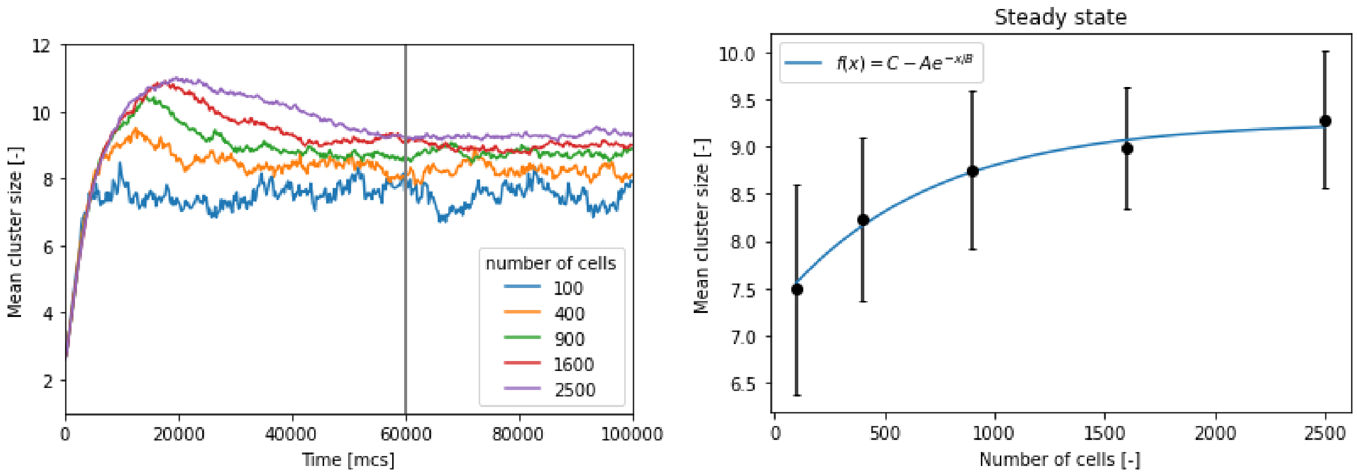


(a)

(b)

Figure S4: Simulation results for different system sizes with $100, 400, 900, 1600$ and 2500 cells. a) Time evolution of the mean cluster size for the various system sizes, including the steady state point $60,000$ mcs. b) Steady state mean cluster size as a function of the number of cells $N$ in the simulations. The result is fitted with an exponential function and the fit value for $C = 9.3 \pm 0.9$, indicating the expected mean cluster size for $N \to \infty$.

# References

[1] Kim JH, Pegoraro AF, Das A, Koehler SA, Ujwary SA, Lan B, et al. Unjamming and collective migration in MCF10A breast cancer cell lines. Biochemical and Biophysical Research Communications. 2020;521(3):706-15. Available from: https://doi.org/10.1016/j.bbrc.2019.10.188.

[2] West AKV, Wullkopf L, Christensen A, Leijnse N, Tarp JM, Mathiesen J, et al. Dynamics of cancerous tissue correlates with invasiveness. Scientific Reports. 2017;7. Available from: https://doi.org/10.1038/srep43800.

[3] Angelini TE, Hannezo E, Trepat X, Marquez M, Fredberg JJ, Weitz DA. Glass-like dynamics of collective cell migration. Proceedings of the National Academy of Sciences (USA). 2011;108(12):4714-9. Available from: https://doi.org/10.1073/pnas.1010059108.
